# Supplementary material for: Convolutional Filtering with RKHS Algebras
Source: arXiv:2411.01341 source file (2025-06-01)
Supplement: Supplementary file 1 [file sec_appendix_paley.tex]

\section{Paley}
\label{sec_appendix_paley}

\begin{example}[Paley Wiener Spaces]\normalfont
\label{exa_rkhs_pw}
Let $\ccalT = \mbR$ and let $\ccalH(K)$ be given by
$
 \ccalH(K) 
   =
   \left\lbrace 
       \left.
          \boldsymbol{f}\in C(\mbR)
       \right\vert 
       \text{supp}\left( \widehat{\boldsymbol{f}} \right) \subset [-W, W]
   \right\rbrace 
   ,
$
where $C(\mbR)$ is the space of continuous functions on $\mbR$ and $\widehat{\boldsymbol{f}}$ is the Fourier transform of $\boldsymbol{f}$. First, we can see that $\ccalH(K)$ is a vector space that can be endowed with the same inner product as in $L_{2}(\mbR)$, i.e.
\begin{equation}
\left\langle 
    \boldsymbol{f},
    \boldsymbol{g}
\right\rangle_{\ccalH(K)}
    =
    \int_{\mbR}\boldsymbol{f}(t)\overline{\boldsymbol{g}(t)}dt
    .
\end{equation}
Taking into account the definition of the inverse Fourier transform we can see that
\begin{equation}
 \boldsymbol{f}(t) 
   =
    \frac{1}{2\pi}
        \int_{-W}^{W}
                \widehat{\boldsymbol{f}}(\omega)e^{j\omega t}
                d\omega
   =
   \frac{1}{2\pi}
    \left\langle
        \widehat{\boldsymbol{f}}
          ,
         e^{-j\omega t}  
    \right\rangle_{\widehat{\ccalH}(W)}
    ,
\end{equation}
where $ \left\langle \cdot , \cdot \right\rangle_{\widehat{\ccalH}(W)}$ is the $L_{2}$ inner product for all the functions supported in $[-W, W]$. Since the Fourier transform defines an isometric transformation we have that
\begin{equation}
 \boldsymbol{f}(t) 
   =
    \frac{1}{2\pi}
    \left\langle
        \widehat{\boldsymbol{f}}
          ,
         e^{-j\omega t} 
    \right\rangle_{\widehat{\ccalH}(W)}
   =
     \left\langle
        \boldsymbol{f}
          ,
        \boldsymbol{k}_{t}
    \right\rangle_{\ccalH(K)}  
    ,
\end{equation}
where 
$
\boldsymbol{k}_{t}(u)
   =
   \frac{W}{\pi}
      \sinc \left( 
                  \frac{W}{\pi}
                        (u-t)
            \right)
            .
$
This is, 
 $
 K(u,t)=   \frac{W}{\pi}
      \sinc \left( 
                  \frac{W}{\pi}
                        (u-t)
            \right)
$
is the reproducing kernel of $\ccalH(K)$. Using the Cauchy-Schwartz inequality, we have that 
\begin{equation}
    \vert \boldsymbol{f}(t) \vert
        \leq 
            \Vert \boldsymbol{f} \Vert_{\ccalH(K)}
            \Vert \boldsymbol{k}_t \Vert_{\ccalH(K)}
            =
            \Vert \boldsymbol{f} \Vert_{\ccalH(K)}
            \sqrt{\frac{W}{\pi}}
            ,
\end{equation}
which guarantees that $\ccalH(K)$ is an RKHS.
\end{example}
